# Supplementary material for: ACACIA: a new method to produce on-the-fly merger trees in the RAMSES code
Source: arXiv:1812.06708 source file (2021-11-23)
Supplement: Supplementary file 1 [file appendix_parallel_algorithm.tex]

%==================================================================================================
\section{Detailed Description of the Parallel Merger Tree Algorithm}\label{app:detailed_mergertree}
%==================================================================================================

The merger tree code starts once clumps have been identified and the 
particle unbinding is completed. The algorithm is designed to work in 
parallel on distributed memory architectures and makes use of the MPI 
standard. When \ramses\ is executed, each processing unit involved in 
the execution is typically referred to by a unique index,  called the 
``MPI rank'', and given a unique domain, i.e. part of the volume of 
the simulated space, to work on. This is simultaneously the advantage,
and the caveat of parallelism on distributed memory architectures:
While we can run codes on a multitude of ranks concurrently and solve
problems that wouldn't fit into the memory of a single rank, ranks 
have no access to other ranks' data, unless the data is explicitly 
communicated.

In what follows, we assume that the code is being executed in parallel 
over multiple MPI ranks. The code then proceeds as follows:

\begin{enumerate}
	\item Write the current clump data to file which is to be read in as 
		progenitor data in the subsequent snapshot:
		For every clump, identify up to $n_{mb}$ tracer particles with 
		minimal binding energy. If a clump consists of less than $n_{mb}$ 
		particles, then take the maximally available number of particles.
		Then write the tracer particles of all ranks into a single shared 
		file. This file will be read in by every rank in once the next 
		snapshot is being processed. If past merged progenitors exist, 
		each rank writes these to (a different) shared file for later use.
	\item Every rank reads in the progenitor data from the shared file 
		of the previous snapshot. It is necessary for each rank to read
		the entire file because between two snapshots particles may leave 
		one rank's domain and be situated	in a different rank's domain. 
		Unfortunately, there is no way to	predict this. 
	
	\item The read in progenitor data is processed:
		First we find which progenitor tracer particles are on each rank's 
		domain by comparing the tracer particles' unique ID to the IDs of 
		the particles currently in this rank's domain.
		Each rank needs to know which tracer particles are currently on its 
		own domain.	Then we find and communicate globally which rank is the 
		``owner'' of which progenitor (and past merged progenitor): 
		The owner of any progenitor is defined as the rank which has the most 
		strongly bound particle of that progenitor within its domain.
		This particle is referred to as the ``galaxy particle'' of this 
		progenitor. Each rank henceforth only keeps track of the tracer 
		particles that are on its domain. The rest are removed from memory.
	
	\item Find links between progenitors and descendants, that is find 
		``which tracer particle ended up where'':
	
		After clump finding, the clump to which any particle belongs is known, 
		and after reading in progenitor data, the progenitor clump 
		to which any tracer particle belonged to is known.
		Each rank now loops through all its local tracer particles.
		Using these two informations (in which clump the particle was and in 
		which clump the particle is now) for every tracer particle, 
		all descendant candidates for all progenitors are found and stored 
		in a sparse matrix, where the rows of the matrix correspond 
		to progenitors and the columns are the descendants.
		The exact number of particle matches between a progenitor-descendant 
		candidate pair is kept.
%		For example: let $n_{mb}=200$. For the progenitor with ID 1, a possible result would be to find 
%50 particles in descendant with ID 2, 120 particles in descendant with ID 7, 10 particles in 
%descendant 3 and 20 particles that aren't in a clump at the current snapshot.
		
		With the sparse matrices populated, they are now communicated across 
		ranks where they are needed. First every rank that has data on 
		progenitors that it doesn't own itself sends this data (specifically, 
		the sparse matrix data) to the owner of that progenitor.
		The owners then gather and sum up all the matches found in the previous 
		linking step for the progenitors that they own and then send them 
		back to any rank that has at least one particle of that progenitor on 
		their domain. (These are the same ranks that sent data to the owner of 
		the progenitor in the first place.)
		
		After communications are done, a transverse sparse matrix is created, 
		where the rows are descendants and the columns are progenitors.
		These matrices will be used to loop through progenitor or descendant 
		candidates.
	
	\item Make trees:
		We first obtain an initial guess for the main progenitors of every 
		descendant and for the main descendant of every progenitor by
		finding the candidate that maximises the merit function given by 
		Equation~\eqref{eq:merit}.
		
		Then we loop to establish matches:
		
		A main progenitor-descendant pair is established when the main 
		progenitor of a descendant is the main descendant of said progenitor,
		or in pseudocode:
		\begin{verbatim}
		match = (main_prog(idesc)==iprog) && 
        (main_desc(iprog)==idesc)
		\end{verbatim}
		
		While there are still descendants without a match and still 
		progenitor candidates left for these descendants:
		
		\begin{itemize}
			
			\item For progenitors without a match: Loop through all 
				descendant candidates. 
				If you find a match, stop there and mark this descendant 
				candidate as the main descendant for this progenitor.
			
			\item Then for all descendants still without a match: 
				Switch to the next best progenitor candidate as current 
				best guess.
			
		\end{itemize}
		
		The loop ends either when all descendants have a match, or 
		if descendants run out of candidates.
		If a progenitor hasn't found a match at this point, we assume 
		that it merged into its best descendant candidate, i.e. the one 
		that maximises the merit function.
	  The merged progenitors are added to the list of past merged 
	  progenitors by adding their ``galaxy particle'' to the list.
		
		If there are descendants that still have no main progenitor,
		we now try finding a progenitor from an older, non-consecutive 
		snapshot. Past merged progenitors are tracked by one particle, 
		their former ``galaxy particle'', which we now refer to as the 
		``orphan particle''.
		All particles of the descendant under investigation are checked 
		for being an orphan particle of a past merged progenitor.
		The most strongly bound orphan particle will be considered the 
		main progenitor of the descendant under consideration.
		If a match is found, the past merged progenitor is removed from 
		the list of past merged progenitors.
		
		Finally, descendants that still haven't found a progenitor at 
		this point are deemed to be newly formed.
		
	\item The results are written to file.

\end{enumerate}
